# Supplementary material for: Nonreciprocal directional dichroism at telecom wavelengths
Source: arXiv:2203.02416 source file (2022-03-04)
Supplement: Supplementary file 1 [file Supplementary_Information_for___Nonreciprocal_directional_dichroism_at_telecom_wavelengths_.pdf]

**Supplementary Information for "Nonreciprocal directional dichroism at telecom wavelengths"**

K. Park *et. al.*

(Dated: February 10, 2022)

**This PDF file includes:**

## Contents

**1. Supplementary Notes** 1

1.1. Symmetry relationships and nonreciprocity in the toroidal geometry of $Ni_3TeO_6$ 1

1.2. Nonreciprocal effects in the raw data 3

1.3. First-principles-based microscopic simulation of nonreciprocal directional dichroism 3

1.4. Comparison between theoretical and experimental nonreciprocity 6

1.5. Vibronic coupling in $Ni_3TeO_6$ 6

1.6. Identifying the phonon sidebands 7

1.7. Phonon side band behavior 7

1.8. Nonreciprocal directional dichroism and the phonon sidebands 10

1.9. Supplementary References 11

# 1. SUPPLEMENTARY NOTES

### 1.1. Symmetry relationships and nonreciprocity in the toroidal geometry of $Ni_3TeO_6$

Supplemental Figure 1 summarizes the nonreciprocal directional dichroism of $Ni_3TeO_6$ over the full set of experimental configurations in the toroidal geometry. As mentioned in the main text, nonreciprocal effects appear when one parameter (either **k** or **H**) is changed thus breaking the relevant symmetries (rotational, inversion, mirror, and time-reversal). Here, we show absorption difference spectra and $\Delta\alpha_{NDD}$ under conditions of different magnetic field direction (with fixed light propagation) as well as changing light propagation direction (with fixed field). There are a total of four permutations. Even though different parameters are swapped, $\Delta\alpha_{NDD}$ (in the green curves) is identical.

Things are different when both light propagation and magnetic field direction are switched because time-reversal symmetry is no longer broken. Supplemental Figure 2 displays the absorption difference spectra of $Ni_3TeO_6$ as well as $\Delta\alpha_{NDD}$ under these conditions. There are two independent examples of reciprocal

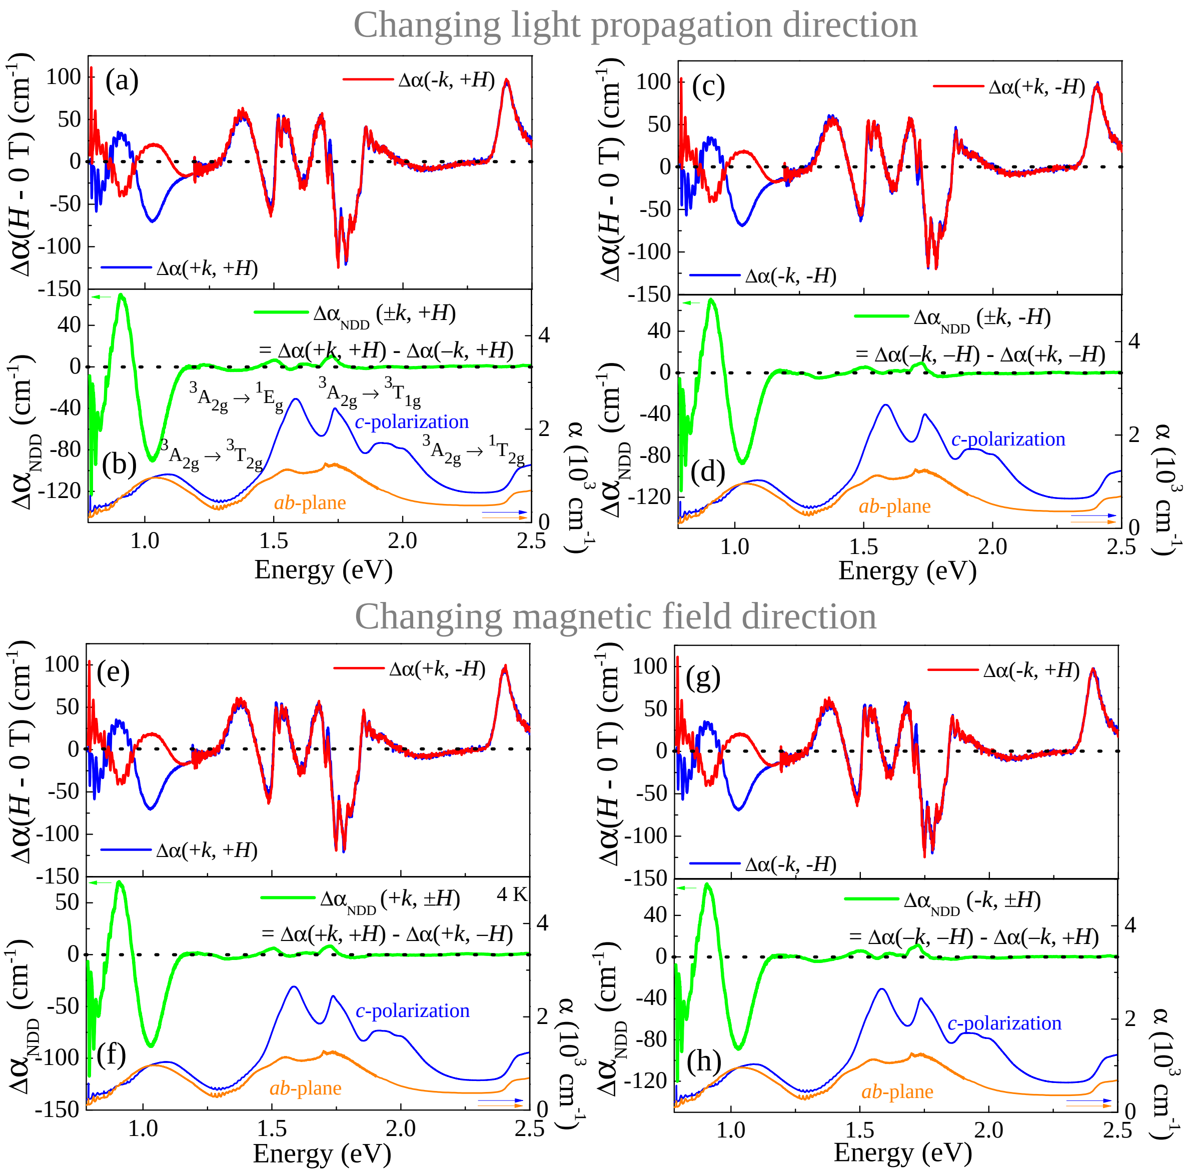


Supplemental Figure 1: (a,c,e,g) Full field absorption difference spectra as a function of energy for several different configurations as indicated. (b,d,f,h) Nonreciprocal directional dichroism is shown in green for four different configurations: $\Delta\alpha_{NDD}$(+**k**, ±**H**), $\Delta\alpha_{NDD}$(±**k**, +**H**), $\Delta\alpha_{NDD}$(-**k**, ±**H**), and $\Delta\alpha_{NDD}$(±**k**, -H), where for instance $\Delta\alpha_{NDD}$(±**k**, +**H**) = $\Delta\alpha$(+**k**, +**H**) - $\Delta\alpha$(-**k**, +**H**). These curves employ **H** = 60 T. The absolute absorption spectrum is included to provide context.

directional dichroism, and in both cases, simultaneous swapping of both **k** and **H** allows time-reversal symmetry to remain intact. As a result, the absorption difference spectra are identical, and $\Delta\alpha_{NDD}$ is zero across the near infrared and visible optics range.

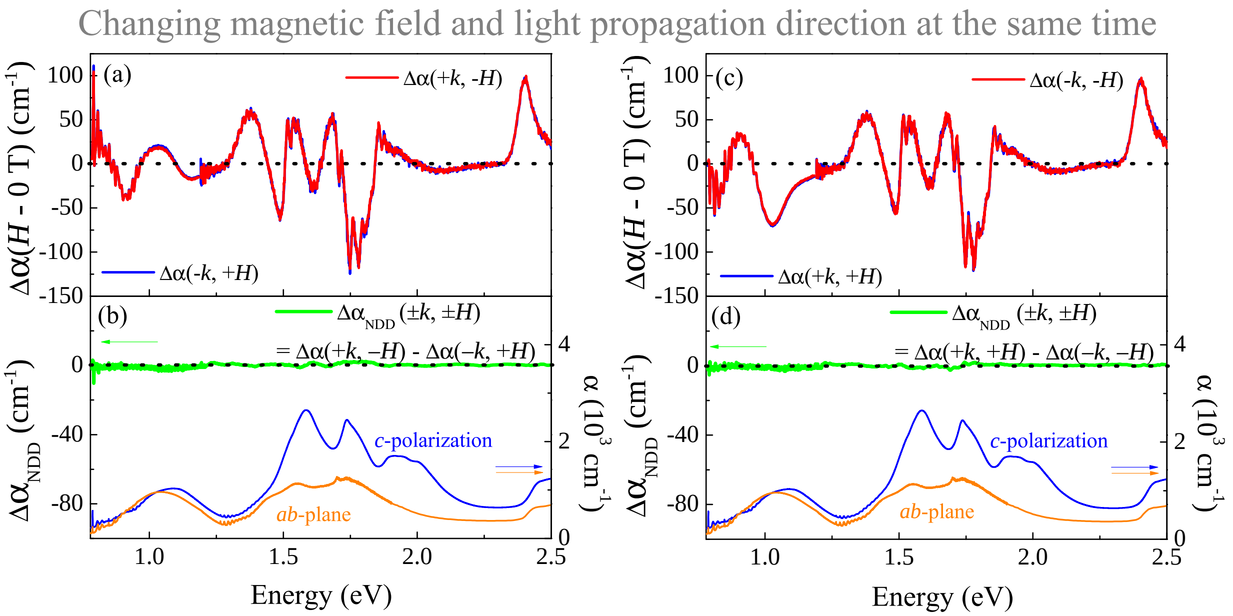


Supplemental Figure 2: (a,c) Full field absorption difference spectra in various configurations. Notice that they are the same. (b,d) $\alpha_{NDD}$ (shown in green) vanishes when both light propagation and magnetic field direction are switched simultaneously. This is because time-reversal symmetry is not broken when the direction of both **k** and **H** are changed together. A magnetic field of 60 T was employed here. The absolute absorption spectrum is shown at the bottom of each panel to provide context.

### 1.2. Nonreciprocal effects in the raw data

Supplemental Figure 3 summarizes the unprocessed, raw power spectra from two different detectors to illustrate the field-induced spectral changes in the absence of any data treatment. Regardless of the exact $\pm\mathbf{k}$ or $\pm\mathbf{H}$ choice, we can see magneto-optical effects in each case. Obviously, the field-induced spectral changes are largest below 1.1 eV - in the InGaS detector regime. Comparison of the panels in Supplemental Fig. 3 reveals the configurations where nonreciprocity appears.

### 1.3. First-principles-based microscopic simulation of nonreciprocal directional dichroism

To simulate $\alpha_{\rm NDD}(\omega) \equiv \alpha_{+}(\omega) - \alpha_{-}(\omega)$ in various geometries, calculations of dielectric, magnetic, and magnetoelectic response tensors of $Ni_3TeO_6$ are needed. In our previous work we have computed the above response tensors employing an *ab-initio*-derived strongly correlated single-ion picture to estimate $\alpha_{\rm NDD}(\omega)$ in the magnetochiral geometry [1]. In this work we extend our previous approach to general situations by

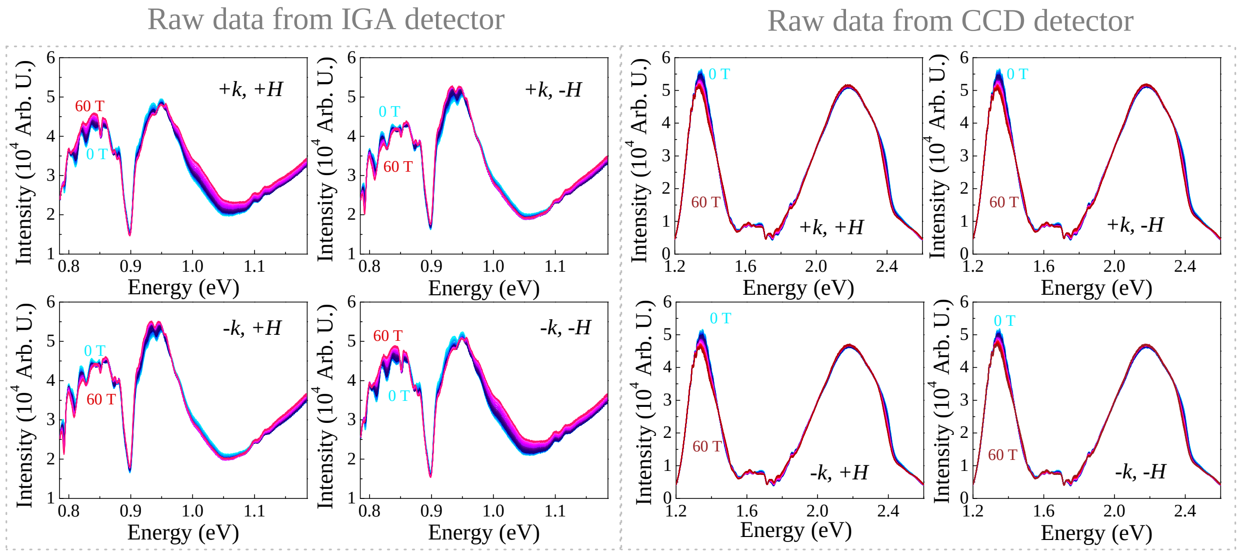


Supplemental Figure 3: Unprocessed power spectra from the two detectors (InGaAs and CCD) from 0 (cyan) to 60 T (red) in various configurations.

solving the following Maxwell's equation including the magnetoelectic tensors,

$$\begin{pmatrix} & & 0 & -1 \\ & & 1 & 0 \\ 0 & 1 & & \\ -1 & 0 & & \end{pmatrix}^{-1} \begin{pmatrix} \epsilon & \chi_{\mathrm{EM}} \\ \chi_{\mathrm{ME}} & \mu \end{pmatrix} \begin{pmatrix} E_x \\ E_y \\ H_x \\ H_y \end{pmatrix} = \frac{1}{v_\sigma(\omega)} \begin{pmatrix} E_x \\ E_y \\ H_x \\ H_y \end{pmatrix}, \qquad (1)$$

where the light propagation direction is set to be along $z$ without losing generality, and $\epsilon$, $\mu$, $\chi_{\mathrm{ME,EM}}$ are 2×2 electric, magnetic, and electro-magnetic (magneto-eletric) response tensors, respectively. Here $v_\sigma(\omega) \equiv \frac{c}{sn_\sigma(\omega)}$ is the phase velocity of light, where $n_\sigma(\omega) \neq 0$ is the complex refractive index of the magnetoelectric medium, and $\sigma \equiv (s, \hat{\mathbf{e}})$ is a compound index embracing polarization ($\hat{\mathbf{e}}$) and light propagation directions ($s = \pm$). Hence $\alpha_{\mathrm{NDD}}(\omega)$ for unpolarized light is readily obtained as a polarization average of $\omega \mathrm{Im}\left[n_{s=+}(\omega) - n_{s=-}(\omega)\right]/c$.

Simulations of magnetic orders under external magnetic fields were performed employing the first-principles-derived magnetic Hamiltonian from Ref. 2. Energy optimizations were done using basin-hopping routines as implemented in the SCIPY package (https://www.scipy.org). First-principles structural optimizations with enforced magnetic configurations mentioned above were done using VASP package as stated in the Method section, after which magnetoelectric tensors were computed employing Ni $d$-multiplets from atomic exact diagonalizations with incorporating crystal fields and spin-orbit coupling.

Supplemental Figure 4 shows a summary of theoretical simulations of nonreciprocal directional dichroism and absorption spectra in three (toroidal, magnetochiral, and transverse magnetochiral) geometries. Note that simulation results generally captures some features observed in experimental $\alpha_{\mathrm{NDD}}$; the strongest

nonreciprocal directional dichroism signal in the toroidal geometry compared to others, and the dominance of $\sim$ 1 eV nonreciprocal directional dichroism signatures in the toroidal geometry (see Fig. 1 in the main text for comparison). Contrary to experimental observations, where the three geometries show the similar order-of-magnitude nonreciprocal directional dichroism responses, about an order of $\sim$ 5 percent of the maximum absorption $\alpha(\omega)$ in the range of $0.5 < \omega < 2.5$ eV, the simulated magnetochiral and transverse magnetochiral geometries show smaller nonreciprocal directional dichroism responses by one order of magnitude compared to the toroidal result (see Supplemental Fig. 4 and Fig. 1 in the main text for comparison).

Note that, in the magnetochiral and transverse magnetochiral geometries, it can be seen via symmetry arguments that bulk electric polarization along the $\hat{z}$-direction does not contribute to the nonreciprocal directional dichroism responses. We also comment that, as mentioned in the main text, the structural chirality of $Ni_3TeO_6$ consists of both local (chiral crystal-field environment at each Ni site) and global (mirror-breaking arrangement of $NiO_6$ octahedra) components. Hence global chirality is likely to be mostly responsible for the nonreciprocal directional dichroism responses in magnetochiral and transverse magnetochiral cases. Since our simulated nonreciprocal directional dichroism is given as a sum of individual Ni atomic contributions, it is likely that the some aspect of global chirality is not captured in our atomic-picture-based simulation in the magnetochiral and transverse magnetochiral cases. Indeed, since each of the three Ni sites in the primitive unit cell belongs to different Wyckoff positions of the $R3$ space group,

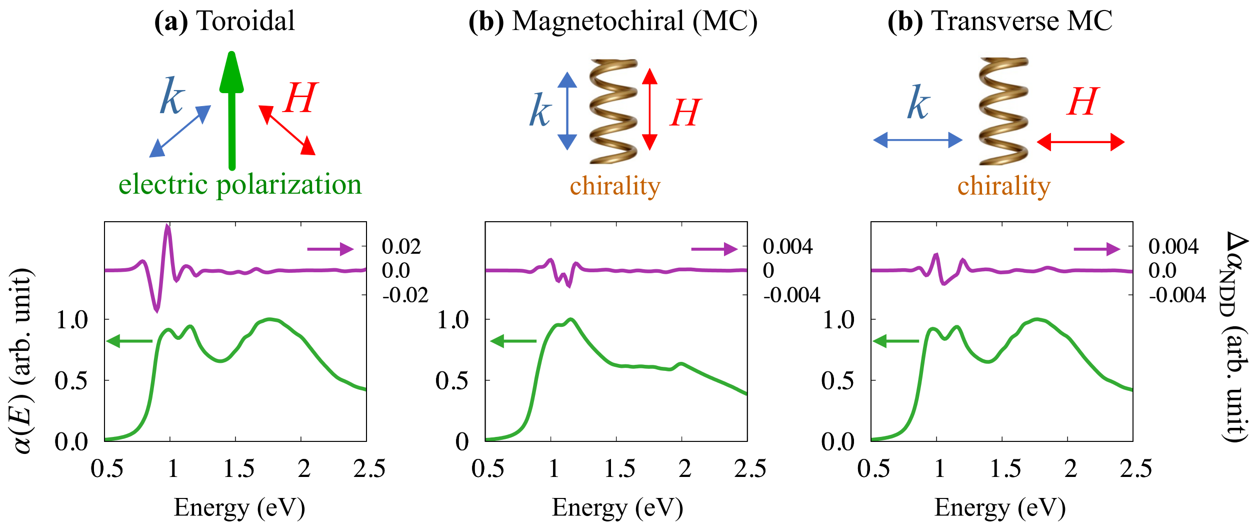


Supplemental Figure 4: Simulated absorption $\alpha(\omega)$ and nonreciprocal $\Delta\alpha_{\mathrm{NDD}}(\omega)$ of (a) toroidal, (b) magnetochiral, and (c) transverse magnetochiral geometries. Note that in each case $\alpha(\omega)$ and $\alpha_{\mathrm{NDD}}(\omega)$ are renormalized with respect to the value of maximum $\alpha(\omega)$ in the given frequency range of $0.5 < \omega < 2.5$ eV. The toroidal and transverse magnetochiral geometries used a simulated magnetic configuration with $\mathbf{H} = 60$ T, whereas the magnetic order of the magnetochiral configuration was obtained with $\mathbf{H} = 66$ T.

simulated atomic nonreciprocal directional dichroism signals from all Ni sites that contribute to the (transverse) magnetochiral nonreciprocal directional dichroism may partially cancel out to yield smaller responses compared to experimental results. On the other hand, since the toroidal nonreciprocal directional dichroism only requires electric and magnetic dipole excitations, the local chiral component that gives rise to the toroidal response is captured in our simulation as shown in Supplemental Fig. 4.

It should also be mentioned that significant nonreciprocal directional dichroism responses in the energy windows of $1.2 < \omega < 2.5$ eV can be only captured in the magnetochiral and transverse magnetochiral geometries. They are almost absent in the toroidal configuration. We speculate that the biggest signature around $\sim 1$ eV originates from both the toroidal and (transverse) magnetochiral components, while excitation in the range of $1.2 < \omega < 2.5$ eV only admits magnetochiral nonreciprocal directional dichroism. Further analyses on this issue may require computational tools properly incorporating both structural chirality and on-site Coulomb correlations, which is beyond the scope of this study.

### 1.4. Comparison between theoretical and experimental nonreciprocity

Supplemental Figure 5 directly compares the measured nonreciprocal directional dichroism in the toroidal configuration with the theoretical simulation. We normalized the simulated spectra in order to match the experimental signal.

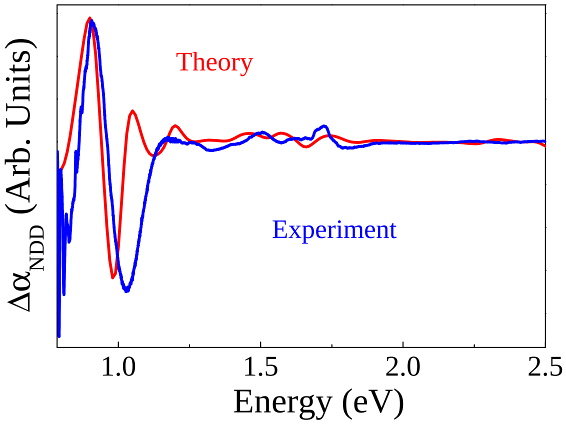


Supplemental Figure 5: A comparison between normalized theoretical and experimental nonreciprocal spectra. The peak maximum was used to normalize the simulated spectra.

### 1.5. Vibronic coupling in $Ni_3TeO_6$

As discussed in Henderson and Imbush [3], the intensity of a zero phonon line goes as $I_0 e^{-S}$, where $S$ is the Huang-Rys factor. Therefore, if $S = 0$, all of the intensity of the electronic excitation is contained in the zero phonon line because there is no shift between the ground and excited state potentials. As $S$ increases, the intensity of the zero phonon line decreases, and at the same time, vibrational "sidebands"

appear at energies $m\hbar\omega$ above the zero phonon excitation. Since oscillator strength is conserved, side band intensity is essentially "borrowed" from the zero phonon line. At sufficiently large $S$, the zero phonon excitation does not appear at all. Rather, the phonon side bands have all of the oscillator strength due to the fact that phonons must be created in the excited state for the excitation to occur. The point is that the weak coupling case ($S$ = small) hosts sharp transitions dominated by the zero phonon line whereas the strong coupling case ($S$ = large) gives broad bands and small or no zero phonon line.

It is well known that transition metal ions are often reasonably well coupled to their crystalline environments. This suggests that $Ni_3TeO_6$ is likely to be in the "strong coupling" limit where $S$ is significantly larger than 1. The experimental spectra of $Ni_3TeO_6$ in Supplemental Fig. 6 are consistent with this supposition: no obvious zero phonon line but reasonably clear phonon side bands - in good agreement with the picture of strong vibronic coupling in this multiferroic.

### 1.6. Identifying the phonon sidebands

Supplemental Figure 6 displays a close-up view of the leading edge of the on-site $Ni^{2+}$ $d$-to-$d$ excitation along with the infrared vibrational spectrum of $Ni_3TeO_6$ [1, 4] positioned underneath for reference. As indicated above, we do not see evidence for a zero phonon line, but we do see phonon sidebands. This is consistent with strong vibronic coupling [3]. For the first progression of phonons, there are five different vibrational modes matching the fine structure in the optical response. These are indicated with dotted black lines. Three separate progressions are shown in Supplemental Fig. 6, and we indicate five different lines in each progression. As expected, the relative intensities and shapes vary, becoming more diffuse at higher energies. Nevertheless, the overall correspondence is clear.

### 1.7. Phonon side band behavior

Supplemental Figure 7(a) displays a close-up view of $\Delta\alpha_{\mathrm{NDD}}$ for the two lowest energy phonon sidebands in the toroidal configuration. Examination reveals that these structures develop systematically and are associated with infrared-active phonons of $Ni_3TeO_6$ at 214 cm$^{-1}$ ($A$ symmetry) and 360 + 370 cm$^{-1}$ ($E$ + $A$ symmetries), respectively [4]. While not every phonon appears in this progression, there is a one-to-one correspondence with those that do appear and those that display nonreciprocal directional dichroism. Focusing on the phonon sideband at 792 meV, we decompose $\Delta\alpha_{\mathrm{NDD}}$ into two absorption difference spectra [Supplemental Fig. 7(b, c)]. To quantify the behavior of these structures, we examined energy and integrated area of the absorption difference spectra $\Delta\alpha$ and the nonreciprocal directional dichroism $\Delta\alpha_{\mathrm{NDD}}$ vs. magnetic field. Our findings are summarized in Supplemental Fig. 7(d, e). There

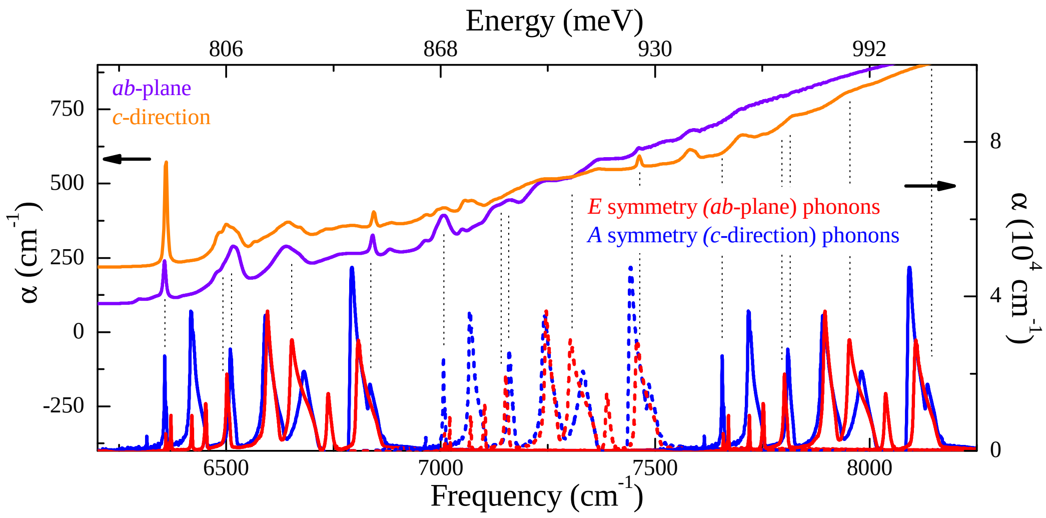


Supplemental Figure 6: Close-up view comparing the phonon sidebands on top of the leading edge of the $Ni^{2+}$ on-site $d$-to-$d$ excitation along with the measured infrared spectrum - repeated sequentially to illustrate the possibility of three different progressions. Black dashed lines match phonons with candidate phonon sidebands.

is a noticeable field-induced shift of the 792 meV feature in $\Delta\alpha_{\rm NDD}$ away from the resonance position of the phonon sideband. The rest of the fine structure shifts in a similar manner. The overall energy scale of the shift is a few meV, consistent with expectations for Zeeman splitting [5], although these measurements were performed with unpolarized light. Moreover, instead of developing linearly with field, there is a slight "kink" between 30 and 35 T. Similar inflection points appear in the magnetostriction, polarization, and magneto-infrared [2, 4] suggesting the possibility of a local lattice distortion in this vicinity. The upper and lower branches of the absorption difference follow suit.

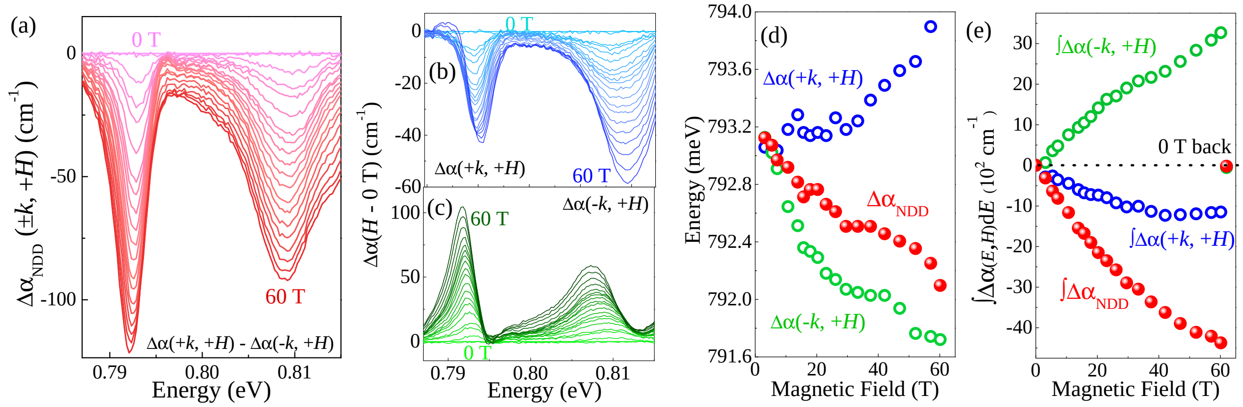


Supplemental Figure 7: (a) Close-up view of $\alpha_{\rm NDD}$ as a function of field between 0 and 60 T. (b, c) Absorption differences, $\Delta\alpha(\mathbf{H}) = \alpha(\mathbf{H})$ - $\alpha(\mathbf{H} = 0$ T). (d) One branch of $\Delta\alpha(\mathbf{H})$ red shifts while the other blue shifts. (e) Integration of $\Delta\alpha(\mathbf{H})$ and $\alpha_{\rm NDD}$ over an appropriate energy window vs. applied field. No hysteresis is observed. Error bars are on the order of the symbol size.

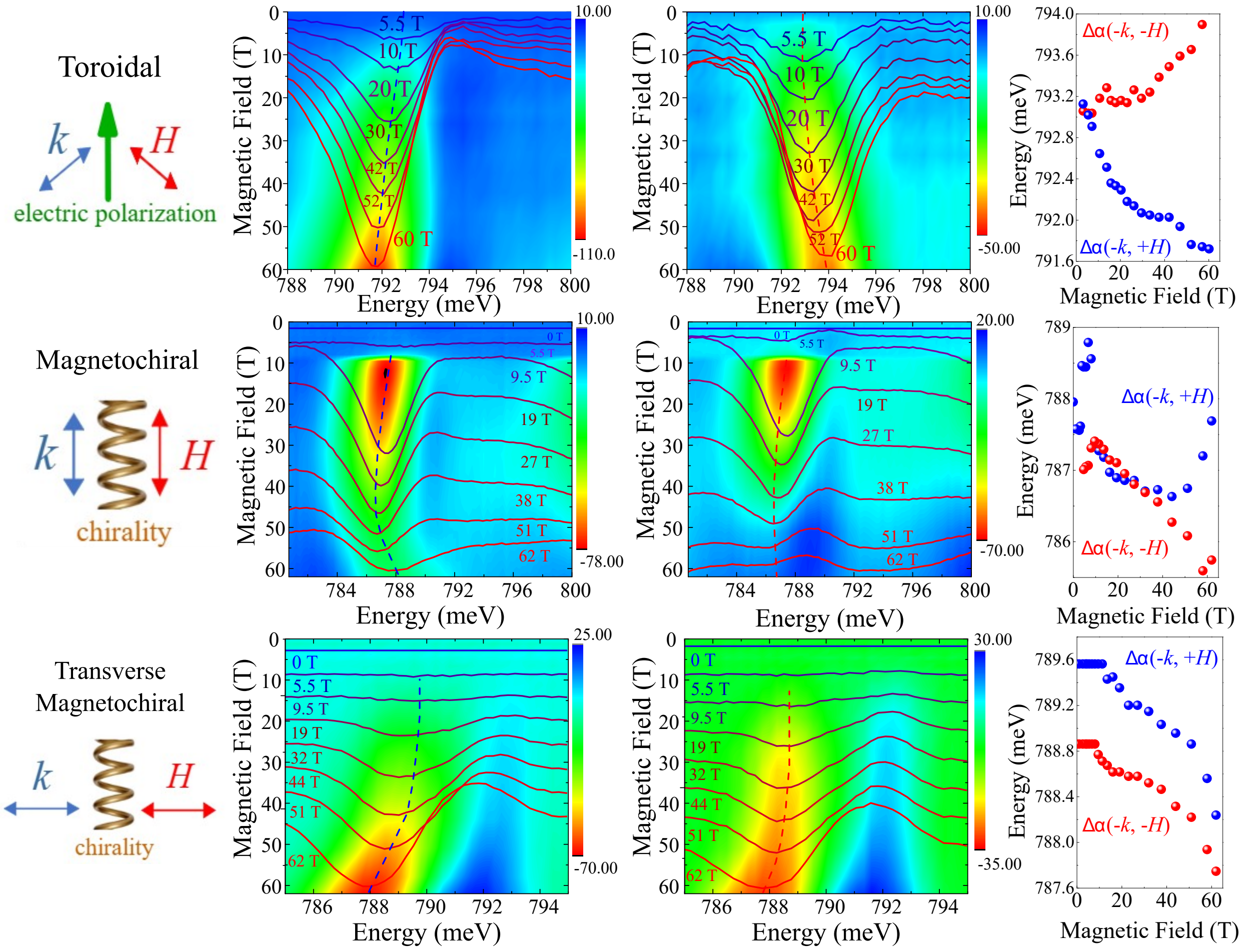


Supplemental Figure 8: Summary of the absorption difference spectra for the first phonon sideband in $Ni_3TeO_6$. The top panels correspond to the toroidal geometry, the middle panels are for the magnetochiral configuration, and the bottom panels correspond to the transverse magnetochiral geometry. Both $\Delta\alpha$(-**k**, +**H**) and $\Delta\alpha$(-**k**, -**H**) are shown as contour plots with the energy on the $x$-axis, magnetic field on the $y$-axis, and spectral intensity on the $z$-axis. The spectra are also plotted on top of the color contour to show the field-induced frequency shift. Frequency shifts vs. applied magnetic field for $\Delta\alpha$(-**k**, +**H**) and $\Delta\alpha$(-**k**, -**H**) are also included.

As we mentioned above, phonon sideband behavior can be tracked more clearly by decomposing the nonreciprocal effect into absorption differences. Supplemental Figure 8 summarizes the absorption difference spectra again, this time focusing on the phonon sideband behavior in the form of a contour plot. These are the components of $\Delta\alpha_{NDD}$. In the toroidal configuration, the lowest energy phonon sideband softens in $\Delta\alpha$(-**k**, +**H**) but hardens in $\Delta\alpha$(-**k**, -**H**) [Supplemental Fig. 8(a,b,c)]. By contrast, the absorption difference components that make up $\Delta\alpha_{NDD}$ in the magnetochiral and transverse magnetochiral geometries shift together - in just one way - from their original position, reinforcing each other to create a $\Delta\alpha_{NDD}$ that shifts systematically. This difference also explains why the absorption difference and $\Delta\alpha_{NDD}$ trends are so complex in the toroidal configuration; the energy shift depends upon the field direction.

Returning briefly to our assignment of the lowest energy phonon sideband at 792 meV as a replica of the 214 $cm^{-1}$ $A$ symmetry phonon in $Ni_3TeO_6$, we can begin to unravel what these trends may imply for the local lattice distortions. This mode has a displacement pattern in which the three Ni ions and the Te center move in an out-of-phase pattern along the $c$-axis [4]. In other words, as Ni(I) moves up, Ni(II) moves down, Ni(III) moves up, and Te moves down. In the toroidal configuration, this excitation shifts strongly depending upon the direction of the applied field, softening in $\Delta\alpha(\text{-}\mathbf{k}, +\mathbf{H})$ and hardening in $\Delta\alpha(\text{-}\mathbf{k}, \text{-}\mathbf{H})$. Magnetostriction [2] may capture these effects as well if the field is pulsed 'up' and 'down'.

### 1.8. Nonreciprocal directional dichroism and the phonon sidebands

Supplemental Figure 9 displays the fine structure on the leading edge of the $Ni^{2+}$ $d$-to-$d$ excitation and shows how these features compare with the sharp detail in $\Delta\alpha_{NDD}$. As discussed in the main text, phonon sidebands ride on top of the $Ni^{2+}$ $d$-to-$d$ excitation; they arise due to vibronic coupling [6]. It is important to note that while not every phonon appears in this progression [Supplemental Fig. 6], there is a one-to-one correspondence with those that do appear in the progression and those that display nonreciprocal directional dichroism. Examination reveals that these structures develop systematically. In the toroidal configuration, contrast begins to appear at the smallest fields because time-reversal symmetry is already broken. As shown in Supplemental Fig. 9, the phonon sidebands of $Ni_3TeO_6$ display nonreciprocal directional dichroism in all three measurement configurations. This is because they have magnetoelectric character. One thing to note is that contrast in the toroidal geometry reveals features that are shifted from their original phonon sideband positions. $\Delta\alpha_{NDD}$ in the other geometries does not show this behavior.

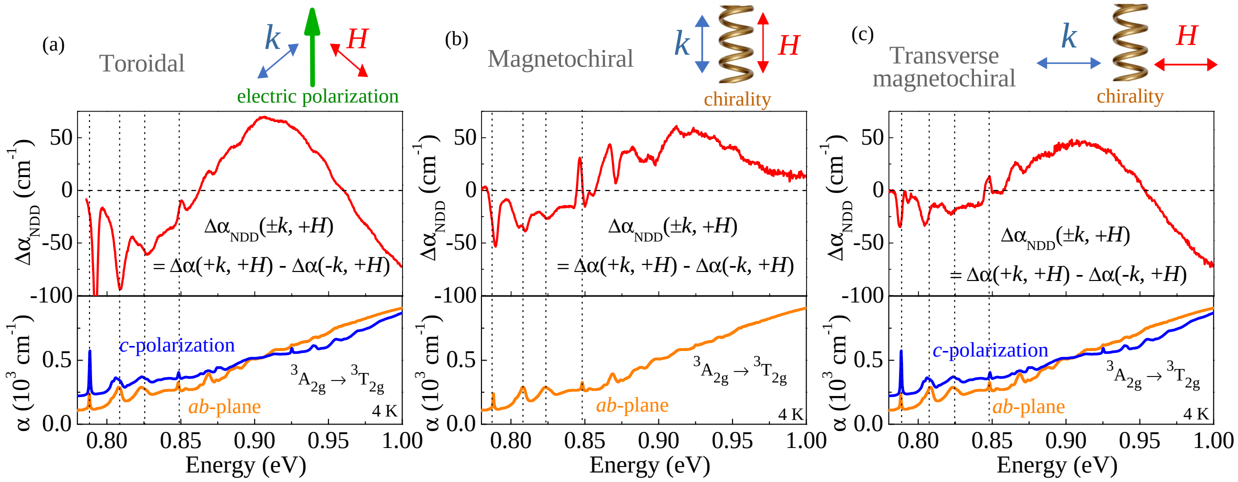


Supplemental Figure 9: Close-up view of the nonreciprocal directional dichroism at full field (60 T) in the toroidal (a), magnetochiral (b), and transverse magnetochiral (c) configurations compared to the phonon side bands in the absolute absorption spectrum. The dark dashed lines denote the position of the fine structure in $\Delta\alpha_{NDD}$. There is a noticeable shift in the toroidal geometry.

## 1.9. Supplementary References


[1] Yokosuk, M. O. *et al.* Nonreciprocal directional dichroism of a chiral magnet in the visible range. *npj Quant. Mater.* **5**, 20 (2020).

[2] Kim, J. W. *et al.* Successive magnetic-field-induced transitions and colossal magnetoelectric effect in $Ni_3TeO_6$. *Phys. Rev. Lett.* **115**, 137201 (2015).

[3] Henderson, B. & Imbusch, G. F. *Optical spectroscopy of inorganic solids* (Oxford [Oxfordshire]; Clarendon Press, 1989).

[4] Yokosuk, M. O. *et al.* Tracking the continuous spin-flop transition in $Ni_3TeO_6$ by infrared spectroscopy. *Phys. Rev. B* **92**, 144305 (2015).

[5] Toyoda, S. *et al.* One-way transparency of light in multiferroic $CuB_2O_4$. *Phys. Rev. Lett.* **115**, 267207 (2015).

[6] Kun, H. & Avril, R. Theory of light absorption and non-radiative transitions in F-centres. *Proceedings of the Royal Society of London. Series A. Mathematical and Physical Sciences* **204**, 406–423 (1950).
